# Supplementary material for: Rethinking Generative Methods for Image Restoration in Physics-based Vision: A Theoretical Analysis from the Perspective of Information
Source: arXiv:2212.02198 source file (2022-12-08)
Supplement: Supplementary file 1 [file 8_appendix.tex]

\section{Information Flow in Generative Deraining Models}

The information bottleneck theory \cite{Information_Bottleneck,Information_Bottleneck_Deep_Learning} explains the training process deep neural networks used for classification or prediction as a process of both

\begin{figure}[!htbp]
    \centering
    \begin{subfigure}{0.48\textwidth}
        \centering
        \begin{tikzpicture}[scale=0.6, every node/.style={scale=0.85}]
            \centering
            \node (Y) at (-2, 0) {$Y$};
            \node (Y_tilde) at (0, 0) {$\tilde{Y}$};
            \node (Z) at (0, 1.5) {$Z$};
            \draw[dashed, -stealth, red, line width=1] (Y) -- (Y_tilde);
            \draw[-stealth, line width=1] (Z) -- (Y_tilde);
            \node at (3, 0) {
                \scalebox{1.2}{
                $\displaystyle
                    \begin{cases}
                      {\color{red}\max I(Y; \tilde{Y})} \\
                      \\
                      {\color{red}\max I(Z; \tilde{Y})} 
                    \end{cases}
                $
                }
            };
        \end{tikzpicture}
        \caption{Original GAN}
        \vspace*{5mm}
    \end{subfigure}
    \hfill
    \begin{subfigure}{0.48\textwidth}
        \centering
        \begin{tikzpicture}[scale=0.6, every node/.style={scale=0.85}]
            \node (Y) at (-2, 0) {$Y$};
            \node (X_tilde) at (0, 0) {$\tilde{X}$};
            \node (Y_tilde) at (2, 0) {$\tilde{Y}$};
            \node (Z) at (2, 1.5) {$Z$};
            \draw[dashed, -stealth, red, line width=1] (Y) -- (-2, -1.5) -- (2, -1.5) -- (Y_tilde);
            \draw[-stealth, line width=1] (Y) -- (X_tilde);
            \draw[-stealth, line width=1] (X_tilde) -- (Y_tilde);
            \draw[-stealth, line width=1] (Z) -- (Y_tilde);
            \node at (5, 0) {
                \scalebox{1.2}{
                $\displaystyle
                    \begin{cases}
                      {\color{red}\max I(Y; \tilde{Y})} \\
                      {\color{red}\max I(Z; \tilde{Y})} \\
                      {\color{red}\max I(\tilde{X}; \tilde{Y})}
                    \end{cases}
                $
                }
            };
        \end{tikzpicture}
        \caption{Conditional GAN (CGAN)}
        \vspace*{5mm}
    \end{subfigure}
    \hfill
    \begin{subfigure}{0.48\textwidth}
        \centering
        \begin{tikzpicture}[scale=0.6, every node/.style={scale=0.85}]
            \node (Y) at (-2, 0) {$Y$};
            \node (X_tilde) at (0, 0) {$\tilde{X}$};
            \node (Y_tilde) at (2, 0) {$\tilde{Y}$};
            \node (X) at (0, 1.5) {$X$};
            \draw[dashed, -stealth, red, line width=1] (Y) -- (-2, -1.5) -- (2, -1.5) -- (Y_tilde);
            \draw[-stealth, line width=1] (Y) -- (X_tilde);
            \draw[-stealth, line width=1] (X_tilde) -- (Y_tilde);
            \draw[-stealth, line width=1] (X) -- (X_tilde);
            \node at (5, 0) {
                \scalebox{1.2}{
                $\displaystyle
                    \begin{cases}
                      {\color{red}\max I(Y; \tilde{Y})} \\
                      {\color{red}\max I(\tilde{X}; \tilde{Y})} \\
                      {\color{blue}\max I(Y; \tilde{X})} \\
                      {\color{blue}\min I(X; \tilde{X})}
                    \end{cases}
                $
                }
            };
        \end{tikzpicture}
        \caption{Image-to-image Translation}
        \vspace*{5mm}
    \end{subfigure}
    \hfill
    \begin{subfigure}{0.48\textwidth}
        \centering
        \begin{tikzpicture}[scale=0.6, every node/.style={scale=0.85}]
            \node (Y) at (-2, 0) {$Y$};
            \node (X) at (0, 0) {$X$};
            \node (Y_tilde) at (2, 0) {$\tilde{Y}$};
            \draw[-stealth, line width=1] (Y) -- (X);
            \draw[-stealth, line width=1] (X) -- (Y_tilde);
            \node at (5, 0) {
                \scalebox{1.2}{
                $\displaystyle
                    \begin{cases}
                      {\color{blue}\max I(Y; \tilde{Y})} \\
                      \\
                      {\color{blue}\min I(X; \tilde{Y})} 
                    \end{cases}
                $
                }
            };
        \end{tikzpicture}
        \caption{Traditional Image De-noising}
        \vspace*{5mm}
    \end{subfigure}
    \hfill
    \begin{subfigure}{0.95\textwidth}
        \centering
        \begin{tikzpicture}[scale=0.6, every node/.style={scale=0.85}]
            \node (Y) at (-3, 0) {$Y$};
            \node (X) at (-1, 0) {$X$};
            \node (X_tilde) at (0, 1.5) {$\tilde{X}$};
            \node (M) at (1, 0) {$M$};
            \node (Y_tilde) at (3, 0) {$\tilde{Y}$};
            \draw[dashed, -stealth, red, line width=1] (Y) -- (-3, -1.5) -- (3, -1.5) -- (Y_tilde);
            \draw[-stealth, line width=1] (Y) -- (X);
            \draw[-stealth, line width=1] (X) -- (X_tilde);
            \draw[-stealth, line width=1] (X_tilde) -- (M);
            \draw[-stealth, line width=1] (X) -- (M);
            \draw[-stealth, line width=1] (M) -- (Y_tilde);
            \node at (6, 0) {
                \scalebox{1.2}{
                $\displaystyle
                    \begin{cases}
                      {\color{red}\max I(Y; \tilde{Y})} \\
                      {\color{red}\max I(M; \tilde{Y})} \\
                      {\color{blue}\max I(Y; M)} \\
                      {\color{blue}\min I(X; M)}
                    \end{cases}
                $
                }
            };
        \end{tikzpicture}
        \caption{Generative Image Deraining}
        \vspace*{5mm}
    \end{subfigure}
    
    \caption{Comparison of Information Flows and Optimization Objectives of Different Models and Tasks}
    \label{fig:excessive_abstraction}
\end{figure}

\section{}
